# Supplementary material for: JPmHC Dynamical Isometry via Orthogonal Hyper-Connections
Source: arXiv:2602.18308 source file (2026-11-08)
Supplement: Supplementary file 1 [file D_numerical_details.tex]

%!TEX root = ../../main.tex

\section{Numerical Implementation Details}\label{app:numerical-details}

This appendix collects the implementation details for the numerical pipelines described in Section~\ref{sec:numerical}.

\subsection{Proof of the $z_1$-mapping (Proposition~\ref{prop:z1-mapping})}\label{app:z1-proof}

\begin{proof}
Denote the single-layer S-transform by $S_1(w)$.
By the definition of the S-transform (Definition~\ref{def:s-transform}), we have the identity
\begin{equation}\label{eq:s-cauchy-relation}
\frac{G_1(z)}{zG_1(z) - 1} = S_1\bigl(zG_1(z) - 1\bigr).
\end{equation}
Setting $w_1 := z_1 G_1(z_1) - 1$, this reads $S_1(w_1) = G_1(z_1) / w_1$.

For $L$ identical layers, the product Cauchy transform $G_L$ satisfies the same structural identity with $S_L = S_1^L$:
\begin{equation}
\frac{G_L(z_L)}{z_L G_L(z_L) - 1} = S_L\bigl(z_L G_L(z_L) - 1\bigr) = S_1\bigl(z_L G_L(z_L) - 1\bigr)^L.
\end{equation}

The key observation is that if we set $w_L := z_L G_L(z_L) - 1 = w_1$ (i.e., we demand that $z_1$ and $z_L$ correspond to the \emph{same} point $w$ in the S-transform domain), then
\begin{equation}
\frac{G_L(z_L)}{w_1} = S_1(w_1)^L = \left(\frac{G_1(z_1)}{w_1}\right)^L,
\end{equation}
so that $G_L(z_L) = w_1 \cdot (G_1(z_1)/w_1)^L = G_1(z_1)^L / w_1^{L-1}$.

From the constraint $z_L G_L(z_L) - 1 = w_1 = z_1 G_1(z_1) - 1$, we obtain
\begin{equation}
z_L = \frac{w_1 + 1}{G_L(z_L)} = \frac{z_1 G_1(z_1)}{G_L(z_L)}.
\end{equation}

Substituting $G_L(z_L) = G_1(z_1)^L / w_1^{L-1}$:
\begin{equation}
z_L = z_1 G_1(z_1) \cdot \frac{w_1^{L-1}}{G_1(z_1)^L} = z_1 \cdot \frac{w_1^{L-1}}{G_1(z_1)^{L-1}} = z_1 \left(\frac{w_1}{G_1(z_1)}\right)^{L-1},
\end{equation}
and since $w_1 = z_1 G_1(z_1) - 1$:
\begin{equation}
z_L = z_1 \left(\frac{z_1 G_1(z_1) - 1}{G_1(z_1)}\right)^{L-1},
\end{equation}
which is the first part of~\eqref{eq:z1-to-zL}. The relation $G_L(z_L) = z_1 G_1(z_1)/z_L$ then follows from $z_L G_L(z_L) = z_1 G_1(z_1)$.
\end{proof}

\subsection{Scalar Dyson solver: analytical derivative}\label{app:scalar-jacobian}

For each spectral parameter $z = x + i\eta$ with $\eta > 0$, we solve~\eqref{eq:dyson-fp} by Newton's method applied to $K(m, z) := \frac{1}{N}\Tr\bigl(A(m)(zI_N - A(m)^\top A(m))^{-1}\bigr) - m = 0$. Writing $R = zI_N - A_m^\top A_m$ where $A_m = A + \sigma^2 m I_N$, the analytical derivative is
\begin{equation}\label{eq:scalar-analytical-jacobian-app}
\frac{dK}{dm} = \frac{\sigma^2}{N}\Bigl[\Tr(R^{-1}) + \Tr\bigl(A_m R^{-1}(A_m^\top + A_m) R^{-1}\bigr)\Bigr] - 1,
\end{equation}
which reuses the already-computed $R^{-1}$ and avoids finite-difference overhead.

\subsection{Matrix-valued Dyson solver}\label{app:matrix-dyson-details}

When the skip connection has the Kronecker structure $A = A_q \otimes I_p$ (Section~\ref{sec:kronecker-skip}), the scalar Dyson equation~\eqref{eq:dyson-fp} is replaced by the $q \times q$ matrix equation~\eqref{eq:matrix-dyson}. We solve this by Newton's method in $\C^{q^2}$.

\medskip
\noindent\textbf{Vectorization.}
Writing $K(M, z) = A_h(zI_q - A_h^\top A_h)^{-1} - M$ as in~\eqref{eq:matrix-dyson}, the Newton update at iterate $M_k$ requires solving
\begin{equation}\label{eq:newton-matrix-dyson-app}
J_k \, \mathrm{vec}(\Delta M) = -\mathrm{vec}(K(M_k, z))
\end{equation}
for $\Delta M \in M_q(\C)$, where $J_k = \partial \mathrm{vec}(K) / \partial \mathrm{vec}(M) \in \C^{q^2 \times q^2}$ is the Jacobian.

\medskip
\noindent\textbf{Analytical Jacobian.}
Let $R = zI_q - A_h^\top A_h$. The Jacobian has the closed form
\begin{equation}\label{eq:analytical-jacobian-app}
J = \sigma^2\bigl(R^{-\top} \otimes I_q\bigr) + \sigma^2\bigl(R^{-\top}A_h^\top \otimes A_h R^{-1}\bigr)\Pi_q + \sigma^2\bigl(R^{-\top} \otimes A_h R^{-1} A_h^\top\bigr) - I_{q^2},
\end{equation}
where $\Pi_q \in \R^{q^2 \times q^2}$ is the \emph{commutation matrix} satisfying $\Pi_q \, \mathrm{vec}(X) = \mathrm{vec}(X^\top)$ for any $X \in M_q(\C)$, and $\otimes$ denotes the Kronecker product of matrices.

\medskip
\noindent\textbf{Damping and initial guesses.}
The Newton step is damped: if $\norm{\Delta M}_F > 10 \max(\norm{M_k}_F, 1)$, the step is rescaled to this bound. The iteration is seeded from multiple initial guesses---$M_0 = 0$, $M_0 = z^{-1}I_q$, $M_0 = (0.05 + 0.05i)I_q$---and the best-converging solution is selected. As in the scalar case, continuation from the previous $z$-point provides the primary seed.\label{rem:branch}

\medskip
\noindent\textbf{Matrix spectral parameter.}
The same Newton procedure extends to the generalized Dyson equation at a matrix spectral parameter $b \in M_q(\C)$:
\begin{equation}\label{eq:dyson-matrix-arg}
K(M, b) := A_h(M) \cdot \bigl(b - A_h(M)^\top A_h(M)\bigr)^{-1} - M = 0,
\end{equation}
by replacing $zI_q$ with $b$ throughout. This is needed for the Psi-inversion in the operator-valued S-transform (Section~\ref{sec:ov-pipeline-numerics}). The Jacobian~\eqref{eq:analytical-jacobian-app} generalizes by substituting $R = b - A_h^\top A_h$.

\subsection{Heterogeneous multi-layer: $w$-domain Newton}\label{app:w-domain}

For $L$ layers with different scalar skip matrices $A^l$ (the case $q = 1$), the S-transform product generalizes to $S_{J^\top J}(w) = \prod_{l=1}^L S_l(w)$, but the $z_1$-mapping (Proposition~\ref{prop:z1-mapping}) no longer applies. Instead, we solve for the common $w$-domain variable.

\medskip
\noindent\textbf{Outer Newton.}
For each target $z_L = x + i\eta$ on the evaluation grid, we seek $w \in \C$ such that
\begin{equation}\label{eq:w-domain-outer-app}
z_L(w) := \frac{w + 1}{w \cdot \prod_{l=1}^L S_l(w)} = z_L^{\mathrm{target}}.
\end{equation}
This is solved by Newton's method on $F(w) := z_L(w) - z_L^{\mathrm{target}} = 0$, with numerical derivative $dF/dw$.

\medskip
\noindent\textbf{Inner Newton.}
Each evaluation of $S_l(w)$ requires solving the scalar Psi-inversion $z_l G_l(z_l) - 1 = w$ for $z_l$, then $S_l(w) = G_l(z_l)/w$. The equation $z G(z) = w + 1$ has a spurious root at $z \to \infty$ where $zG(z) \to 1$; the Newton solve is therefore seeded at $z_l^{(0)} = z_L^{\mathrm{target}}$ (the physical branch) rather than the naive guess $(w+1) \cdot 1.05$.

\medskip
\noindent\textbf{Recovery and continuation.}
Once $w$ is found, $G_L(z_L) = (w + 1)/z_L$. All state---the outer $w$ and the inner $(z_l, m_l)$ for each layer---is carried forward to the next grid point, providing warm starts that maintain branch tracking across the $z$-grid. The outer step is damped: $\abs{\Delta w}$ is capped at $10 \max(\abs{w}, 1)$.

\subsection{Operator-valued pipeline: implementation}\label{app:ov-pipeline}

For $L > 1$ heterogeneous layers with $q > 1$, the full operator-valued pipeline involves a \emph{triple-nested Newton} structure.

\medskip
\noindent\textbf{Level 1: Outer Newton on $W \in M_q(\C)$.}
For each target $z = x + i\eta$, we solve the consistency equation~\eqref{eq:outer-consistency} by Newton's method on $q^2$ complex unknowns. The residual is
\begin{equation}\label{eq:ov-outer-residual-app}
F(W) = (W + I_q)\bigl(S_{\mathrm{prod}}(W) \cdot W\bigr)^{-1} - z I_q \in M_q(\C),
\end{equation}
with the Jacobian $\partial \mathrm{vec}(F)/\partial \mathrm{vec}(W) \in \C^{q^2 \times q^2}$ computed by $q^2$ finite-difference perturbations, each requiring a full evaluation of $S_{\mathrm{prod}}(W)$.

\medskip
\noindent\textbf{Level 2: Twisted S-product.}
Each evaluation of $S_{\mathrm{prod}}(W)$ computes the $L$-fold twisted recursion~\eqref{eq:twisted-fold}, calling $S_l^{(\mcB)}(W_{\mathrm{twisted}})$ once per layer.

\medskip
\noindent\textbf{Level 3: Psi-inversion per layer.}
Each $S_l^{(\mcB)}$ evaluation requires solving the Psi-inversion~\eqref{eq:psi-inversion} for $b_l \in M_q(\C)$, which itself invokes the matrix-argument Dyson solver (Section~\ref{app:matrix-dyson-details}).

\medskip
\noindent\textbf{Backtracking line search.}
The outer Newton step $\Delta W$ is accepted with step size $\alpha \in \{1, 0.5, 0.25, 0.1, 0.05, 0.02, 0.01\}$, choosing the largest $\alpha$ such that $\norm{F(W + \alpha \Delta W)}_F < \norm{F(W)}_F$ and all inner solves (Levels 2--3) converge.

\medskip
\noindent\textbf{Warm-starting and continuation.}
The per-layer Psi-inversion solutions $(b_l, M_l)$ are cached across both Newton iterations (within a single $z$-point) and across consecutive $z$-points, enabling effective continuation. The initial guess for $b_l$ is selected from a hierarchy:
\begin{enumerate}
\item \emph{Continuation hint}: the cached $b_l$ from the previous solve;
\item \emph{Scalar Newton}: find $z$ such that $z G_{\mathrm{scalar}}(z) = \frac{1}{q}\Tr(W + I_q)$, then set $b = zI_q$;
\item \emph{Per-sector diagonal hint} (when $A_q$ is diagonal): solve $q$ independent scalar Psi-inversion problems, one per diagonal entry of $A_q$;
\item \emph{Asymptotic fallback}: $b = W + I_q$.
\end{enumerate}

\subsection{Parallelism}\label{app:parallelism}

The evaluation grid $\{z_k = x_k + i\eta\}_{k=1}^K$ is split into $n_{\mathrm{jobs}}$ contiguous chunks for parallel processing.

\medskip
\noindent\textbf{Sequential pre-sweep.}
To initialize each chunk with a valid warm start, the first $z$-point of each chunk is solved \emph{sequentially} in order, carrying the full continuation state $(W, \{b_l, M_l\}_{l=1}^L)$ from chunk to chunk. Without this pre-sweep, cold-starting a chunk at a $z$-point deep inside the spectral support would require the full initial-guess hierarchy and may converge to the wrong branch.

\medskip
\noindent\textbf{Parallel dispatch.}
After the pre-sweep, each chunk is dispatched to a separate process via \texttt{ProcessPoolExecutor}. Thread-level parallelism (\texttt{ThreadPoolExecutor}) is avoided because the BLAS routines for small $q \times q$ matrices do not release the GIL.

\subsection{Monte Carlo validation}\label{app:mc-validation}

Theoretical predictions are validated by direct Monte Carlo sampling.

\medskip
\noindent\textbf{Single layer.}
For each sample $s = 1, \ldots, n_{\mathrm{MC}}$: draw $W^{(s)}$ with i.i.d.\ $\mathcal{N}(0, 1/N)$ entries, form
\begin{equation}
Y^{(s)} = (A_q \otimes I_p) + D^{(s)} W^{(s)},
\end{equation}
and compute the eigenvalues of $(Y^{(s)})^\top Y^{(s)}$ via a symmetric eigensolver. Here $D^{(s)} = \mathrm{diag}(\phi'(\sqrt{q^l} \, z_i))$ with $z_i \sim \mathcal{N}(0,1)$ for nonlinear activations, or $D^{(s)} = \sqrt{\sigma^2}\, I_N$ for the linear case.

\medskip
\noindent\textbf{Multi-layer.}
The Jacobian $J^{(s)} = \prod_{l=1}^L Y_l^{(s)}$ is formed by multiplying $L$ independent layer matrices, and the eigenvalues of $(J^{(s)})^\top J^{(s)}$ are computed. The empirical spectral density is obtained by histogramming the pooled eigenvalues across all samples with \texttt{density=True} normalization.

\subsection{Activation moments and signal propagation}\label{app:signal-prop}

The self-energy $\sigma^2$ entering the Dyson equation depends on the activation function $\phi$ and the signal propagation dynamics across layers.

\medskip
\noindent\textbf{Moment computation.}
The key activation moments are computed by Gauss--Hermite quadrature~\cite{golub1969calculation} (probabilists' Hermite polynomials, $n_{\mathrm{nodes}} = 100$):
\begin{equation}\label{eq:activation-moments-app}
\psi(v) = \E\bigl[\phi'(\sqrt{v}\, Z)^2\bigr], \quad \kappa(v) = \E\bigl[\phi(\sqrt{v}\, Z)^2\bigr], \quad Z \sim \mathcal{N}(0, 1).
\end{equation}

\medskip
\noindent\textbf{Signal propagation recursion.}
Given weight variance $\sigma_w^2$ and per-layer twist matrices $A_q^l$, the pre-activation variance $q^l$, self-energy $\sigma^2_l$, and signal variance $v^l$ propagate as
\begin{equation}\label{eq:signal-prop-app}
q^l = \sigma_w^2\,(v^{l-1} + \sigma^2_{l-1}), \quad \sigma^2_l = \psi(q^l), \quad v^l = \kappa(q^l) + \frac{\norm{A_q^l}_F^2}{q}\, v^{l-1}.
\end{equation}
The Dyson input is $\sigma^2_l = \sigma_w^2 \cdot \psi(q^l)$, and the critical dynamical isometry condition (Section~\ref{sec:dyson-resnet}) generalises to $L \sigma^2 = 1/2$ for identical layers.
