# Supplementary material for: JPmHC Dynamical Isometry via Orthogonal Hyper-Connections
Source: arXiv:2602.18308 source file (2026-11-08)
Supplement: Supplementary file 2 [file E_spectral_stalling.tex]

%!TEX root = ../../main.tex

\section{Spectral Stalling: From Jacobian Spectrum to Optimiser Dynamics}\label{app:spectral-stalling}

The main text analyses the \emph{shape} of the Jacobian spectrum as a function of the skip-connection matrix $A_q$. This appendix addresses the complementary question: how does that spectral shape affect gradient-based training? We argue that four independent mechanisms each impose a \emph{hard cutoff} $\sigma^*$ on the singular-value spectrum, below which gradient directions are operationally invisible to the optimiser. The binding cutoff is
\begin{equation}\label{eq:sigma-star}
\sigma^* = \max\!\bigl(\sigma^*_{\mathrm{time}},\; \sigma^*_{\mathrm{Adam}},\; \sigma^*_{\mathrm{bf16}},\; \sigma^*_{\mathrm{noise}}\bigr).
\end{equation}
Below $\sigma^*$, the network trains in a subspace of effective dimension $n_{\mathrm{eff}} = n\!\int_{\sigma^*}^{\infty}\!d\mu_\Sigma(\sigma)$. We call this \emph{spectral stalling}, by analogy with aerodynamic stall: beyond a critical threshold, the gradient in a given direction no longer produces useful lift.

\subsection{Setup: spectral filtering of the backward pass}\label{app:stalling-setup}

The backward error signal at layer $l$ is $\delta_l = J_{l\to L}^\top \,\nabla_{\mathbf{h}_L}\!\mathcal{L}$, where $J_{l\to L} = \prod_{k=l+1}^{L} J_k$ with $J_k = D_k W_k + A_k$. Decomposing in the SVD $J_{l\to L} = U\Sigma V^\top$:
\begin{equation}\label{eq:spectral-filtering}
\delta_l = V\,\Sigma\,U^\top\,\nabla_{\mathbf{h}_L}\!\mathcal{L}, \qquad (\delta_l)_i = \sigma_i\,\alpha_i, \quad \alpha = U^\top\nabla\mathcal{L}.
\end{equation}
Each component of the loss gradient is multiplied by the corresponding singular value~$\sigma_i$. Directions with $\sigma_i \approx 0$ receive no gradient information. This is not the classical vanishing-gradient problem (which concerns the \emph{mean} of $\sigma$); it is a \emph{directional filtering} that depends on the full spectral measure~$\mu_\Sigma$.

\subsection{Cutoff I: exponential timescale separation}\label{app:cutoff-time}

Saxe, McClelland, and Ganguli~\cite{saxe2014exact} solved the gradient-flow dynamics of deep linear networks in closed form. In the SVD basis of the input--output correlation, each singular mode $i$ evolves with a sigmoidal trajectory whose time constant satisfies $\tau_i \propto 1/\sigma_i(0)$. Modes with small $\sigma_i$ take exponentially longer to converge; after a training budget of $T$ steps, only modes with $\tau_i \lesssim T$ have appreciably moved.

This yields a finite-time cutoff:
\begin{equation}\label{eq:sigma-time}
\sigma^*_{\mathrm{time}} \;\sim\; \frac{C}{T\,\eta\,\sigma_{\max}},
\end{equation}
where $C$ depends on the loss landscape curvature. Relative to the dominant mode, the number of steps to halve the error in direction $i$ scales as $t_{1/2}^{(i)} / t_{1/2}^{(\max)} = (\sigma_{\max}/\sigma_i)^2$~\cite{jacot2018ntk}. A mode with $\sigma_i = 0.01\,\sigma_{\max}$ requires $10^4\times$ more steps---it is simply not reached within any practical training budget.

Arora et al.~\cite{arora2019implicit} showed that gradient descent with small initialisation has an implicit bias toward low-rank solutions: $\dot{\sigma}_i \propto \sigma_i^{2-2/N}$, so large singular values accelerate while small ones stagnate. Pesme and Flammarion~\cite{pesme2023saddle} made this precise for diagonal linear networks: gradient flow sequentially jumps from saddle to saddle, each corresponding to the activation of a new singular mode, with jump times computable via a recursive algorithm.

\subsection{Cutoff II: Adam's $\epsilon$-threshold}\label{app:cutoff-adam}

Adam~\cite{kingma2015adam} maintains running estimates $m_i \approx \mathbb{E}[g_i]$ and $v_i \approx \mathbb{E}[g_i^2]$ of the gradient in each coordinate, with normalised update $m_i/(\sqrt{v_i} + \epsilon)$. Balles and Hennig~\cite{balles2018dissecting} showed this ratio is essentially the signal-to-noise ratio of $g_i$. In the regime $\sigma_i |\alpha_i| \ll \epsilon$, the update becomes $\sigma_i \alpha_i / \epsilon$, which vanishes linearly in $\sigma_i$:
\begin{equation}\label{eq:sigma-adam}
\sigma^*_{\mathrm{Adam}} \;\sim\; \frac{\epsilon}{|\bar\alpha|},
\end{equation}
where $\bar\alpha$ is the typical loss-gradient component. With the standard $\epsilon = 10^{-8}$, this cutoff is rarely binding in practice---the other floors kick in first.

A structural limitation prevents Adam from compensating for spectral filtering: Adam operates \emph{per-parameter} (in the weight-matrix coordinate system), but the spectral filtering operates in the \emph{Jacobian singular-vector basis}, which is a rotation of the parameter basis that changes with the input. Zhang et al.~\cite{zhang2024adam} demonstrated this directly: ViT training degrades under random global rotations of the parameter space, even though the optimisation landscape is unchanged. Adam's advantages are \emph{representation-dependent}, not universal~\cite{depavia2025rotations}.

\subsection{Cutoff III: low-precision arithmetic (bf16 swamping)}\label{app:cutoff-bf16}

BFloat16 has a relative precision of $u_{\mathrm{bf16}} = 2^{-8} \approx 3.9 \times 10^{-3}$. When accumulating a gradient update $\Delta w$ into a weight $w$, if $|\Delta w| < u_{\mathrm{bf16}} \cdot |w|$, the update is \emph{swamped}: $\mathrm{fl}(w + \Delta w) = w$ exactly. The gradient is lost to rounding. Since the gradient update in direction $i$ scales as $\eta \sigma_i |\alpha_i|$:
\begin{equation}\label{eq:sigma-bf16}
\sigma^*_{\mathrm{bf16}} \;\sim\; \frac{u_{\mathrm{bf16}}\,|w|}{\eta\,|\bar\alpha|}.
\end{equation}
With $\eta = 10^{-4}$, $|w| \sim 1$, $|\bar\alpha| \sim 1$: $\sigma^*_{\mathrm{bf16}} \sim 40$. This is an aggressive cutoff---in bf16 without loss scaling, only the dominant singular directions receive non-zero updates.

Loss scaling~\cite{micikevicius2018mixed} extends the dynamic range of the gradient but does not increase relative precision: the ratio $\sigma_i/\sigma_j$ is preserved after scaling. It helps with gradient \emph{underflow} but not with accumulation swamping. Stochastic rounding~\cite{gupta2015limited} softens the hard cutoff to a probabilistic one (preserving small updates in expectation), but the effective learning rate in low-$\sigma$ directions is still drastically reduced because stochastic-rounding variance overwhelms the signal~\cite{zamirai2020bfloat16}.

\subsection{Cutoff IV: stochastic noise floor}\label{app:cutoff-noise}

For mini-batch SGD with batch size $B$, the stochastic gradient in singular direction $i$ has mean $\sigma_i \bar\alpha_i$ and variance $\sigma_i^2 \operatorname{Var}(\alpha_i) / B$. The signal-to-noise ratio $\mathrm{SNR}_i = |\bar\alpha_i|\sqrt{B}/\mathrm{std}(\alpha_i)$ is independent of $\sigma_i$. However, the relative update magnitude in direction $i$ compared to the dominant direction is $\sigma_i / \sigma_{\max}$, regardless of noise. When $\sigma_i / \sigma_{\max} \ll 1$, the cumulative displacement in direction $i$ is negligible, giving:
\begin{equation}\label{eq:sigma-noise}
\sigma^*_{\mathrm{noise}} \;\sim\; \frac{\sigma_{\max}}{\mathrm{SNR}_{\max}} \cdot \frac{1}{\sqrt{B}}.
\end{equation}
This cutoff is alleviated by increasing batch size and is typically subdominant to the bf16 and timescale floors.

\subsection{The unified picture}\label{app:stalling-unified}

In typical modern training (Adam, bf16, batch size 256--4096, $T \sim 10^5$ steps), the four cutoffs have the following typical magnitudes:

\begin{center}
\begin{tabular}{lll}
\toprule
Cutoff & Expression & Typical order \\
\midrule
$\sigma^*_{\mathrm{time}}$ & $C / (T\eta\sigma_{\max})$ & $10^{-2}$--$10^{-1}$ \\
$\sigma^*_{\mathrm{Adam}}$ & $\epsilon / |\bar\alpha|$ & $10^{-4}$--$10^{-3}$ (rarely binding) \\
$\sigma^*_{\mathrm{bf16}}$ & $u_{\mathrm{bf16}}|w| / (\eta|\bar\alpha|)$ & $10^{-2}$--$10^{1}$ (\textbf{often dominant}) \\
$\sigma^*_{\mathrm{noise}}$ & $\sigma_{\max}/(\mathrm{SNR}_{\max}\sqrt{B})$ & $\sim 10^{-2}$ \\
\bottomrule
\end{tabular}
\end{center}

\noindent The bf16 swamping floor and the finite-time horizon are typically the binding constraints. This hierarchy means that spectral collapse in the Jacobian has direct, quantitative consequences for training: singular-value mass below $\sigma^*$ corresponds to capacity that the optimiser cannot access.

\subsection{Why only natural gradient could compensate}\label{app:natural-gradient}

The natural gradient update $\Delta\theta = -\eta\, F^{-1}\nabla_\theta\mathcal{L}$, where $F = \mathbb{E}[J_\theta^\top J_\theta]$ is the Fisher information (Gauss--Newton approximation), satisfies $F^{-1}\nabla\mathcal{L} = (\alpha_1, \ldots)$ in the Jacobian singular basis---the spectral filtering is \emph{exactly inverted}~\cite{amari1998natural}. Each direction receives a step proportional to $\alpha_i$ alone, independent of $\sigma_i$. This is why natural gradient converges at a rate independent of the condition number.

Adam approximates a \emph{diagonal} preconditioner in the \emph{parameter coordinate system}. The diagonal approximation discards the off-diagonal structure that couples parameters within a singular direction. Das et al.~\cite{das2024preconditioning} showed that Adam's effective condition number is $\mathcal{O}(\min(d, \kappa))$ for diagonal Hessians but offers no improvement for non-diagonal ones---precisely the case when spectral filtering operates in a rotated basis. K-FAC~\cite{martens2015kfac} and Shampoo~\cite{gupta2018shampoo} achieve partial spectral inversion via Kronecker-factored or per-dimension preconditioners, but neither fully inverts the Jacobian filtering. The hierarchy is: natural gradient (exact inversion) $>$ K-FAC/Shampoo (partial) $>$ Adam (coordinate-wise only) $>$ SGD (none).

\subsection{Connections to our spectral analysis}\label{app:stalling-connections}

\noindent\textbf{Computable stalling fraction.}
Our operator-valued Dyson pipeline gives the spectral measure $\mu_\Sigma$ as a function of the skip-connection matrix $A_q$, the weight variance $\sigma_w^2$, the activation function $\phi$, and depth $L$. Combined with the stalling threshold $\sigma^*$ from~\eqref{eq:sigma-star}, this yields a concrete, computable prediction for the stalling fraction:
\begin{equation}\label{eq:stalling-fraction}
\rho_{\mathrm{stall}}(A_q, L, \sigma^*) = \int_0^{\sigma^*} d\mu_\Sigma(\sigma).
\end{equation}

\noindent\textbf{Depth scaling.}
For doubly stochastic $A_q$ with interior eigenvalue $|\lambda_j| < 1$, the spectral measure develops a growing lower tail as $L$ increases, because the contribution of each contracting sector to the Jacobian decays as $|\lambda_j|^L$. The stalling fraction $\rho_{\mathrm{stall}}$ therefore increases with depth: \emph{deeper doubly stochastic networks stall in more directions}. For orthogonal $A_q \in O(q)$, all eigenvalues lie on the unit circle, the spectrum does not develop a lower tail, and $\rho_{\mathrm{stall}}$ remains small at all depths.

\medskip
\noindent\textbf{The bf16 interaction.}
The bf16 cutoff is particularly relevant for our setting because modern transformer training universally uses bf16 or fp16 mixed precision. Our spectral analysis can predict \emph{which} skip-connection structures produce spectra that fall below the bf16 swamping floor. If $\mu_\Sigma$ places significant mass in $[0, \sigma^*_{\mathrm{bf16}}]$, then bf16 training of that architecture will be effectively lower-dimensional---a prediction testable by comparing bf16 vs.\ fp32 training of networks with different skip-connection matrices.
