# Supplementary material for: JPmHC Dynamical Isometry via Orthogonal Hyper-Connections
Source: arXiv:2602.18308 source file (2026-11-08)
Supplement: Supplementary file 3 [file implementation.tex]

% ============================================================
% Section 8: Implementation Details
% ============================================================
\section{Implementation Details}
\label{sec:implementation}

This section describes the engineering decisions and optimizations that make our JPmHC variants production-ready for distributed training.

\subsection{Fused Phi Projections}

A na\"ive implementation would use three separate linear layers for $\phi_{\text{pre}}$, $\phi_{\text{post}}$, and $\phi_{\text{res}}$. Since all three share the same input $\bx_{\text{norm}} \in \R^{nd}$, we \textbf{fuse} them into a single projection:
\begin{equation}
  \begin{bmatrix} \phi_{\text{pre}} \\ \phi_{\text{post}} \\ \phi_{\text{res}} \end{bmatrix}
  = \bW_{\text{fused}} \cdot \bx_{\text{norm}} + \mathbf{b}_{\text{fused}},
  \quad \bW_{\text{fused}} \in \R^{(n + n + D_{\text{res}}) \times nd},
  \label{eq:fused-phi}
\end{equation}
where $D_{\text{res}}$ depends on the variant:
\begin{itemize}[leftmargin=2em]
  \item \textbf{Sinkhorn}: $\phi_{\text{pre}} \in \R^n$, $\phi_{\text{post}} \in \R^n$, $\phi_{\text{res}} \in \R^{n^2}$; total output dim $= 2n + n^2$,
  \item \textbf{Cayley}: All three outputs are $n \times n$ matrices (pre, post, res); total output dim $= 3n^2$. Pre/post use softmax (row/column-stochastic), not sigmoid.
  \item \textbf{Grassmann}: $\phi_{\text{pre}} \in \R^n$, $\phi_{\text{post}} \in \R^n$, $\phi_{\text{res}} \in \R^{np}$; total output dim $= 2n + np$,
  \item \textbf{Perm Mix}: $\phi_{\text{pre}} \in \R^n$, $\phi_{\text{post}} \in \R^n$, $\phi_{\text{mix}} \in \R^K$; total output dim $= 2n + K$.
\end{itemize}

This fusion reduces memory bandwidth by a factor of $\sim$$3\times$ (one \texttt{GEMM} instead of three), which is significant in bandwidth-bound regimes at small batch sizes.

\subsection{Custom Triton Kernels}
\label{sec:triton-kernels}

All manifold projections and their backward passes are implemented as custom Triton~\citep{tillet2019triton} kernels, operating entirely in scalar registers for the $n = 4$ case. This eliminates the overhead of launching dozens of small CuBLAS \texttt{GEMM}s and enables fusion of multi-step iterative algorithms into single kernel launches.

\begin{table}[h]
\centering
\caption{Custom Triton kernels and their PyTorch-equivalent launch counts.}
\label{tab:triton-kernels}
\begin{tabular}{llc}
\toprule
Kernel & Operation & Replaces \\
\midrule
\texttt{cayley\_n4} & Skew decomposition $+$ iterative Cayley map (fwd) & $\sim$13 kernels \\
\texttt{sinkhorn\_logspace\_n4} & 20 log-space row/col normalization iters (fwd) & $\sim$40 kernels \\
\texttt{sinkhorn\_implicit\_bwd\_n4} & 16-iter Gauss--Seidel implicit diff (bwd) & $\sim$32 kernels \\
\texttt{fused\_mhc\_cayley\_n4} & softmax(pre) $+$ softmax(post) $+$ Cayley(res) & $\sim$15 kernels \\
\texttt{grassmann\_softmax\_n4} & softmax(pre) $+$ softmax(post) for Grassmann & $\sim$6 kernels \\
\texttt{grassmann\_qr\_n4} & Modified Gram--Schmidt retraction on $\Stiefel(n,p)$ & 2 cuSOLVER calls \\
\bottomrule
\end{tabular}
\end{table}

All $4 \times 4$ matrix operations (multiplications, inversions, softmax reductions) are fully unrolled in registers, avoiding shared memory entirely. The Sinkhorn backward kernel implements the Gauss--Seidel solver from \Cref{eq:implicit-grad} directly in-kernel, performing 16 coupled iterations without intermediate global memory writes. The Grassmann QR kernel performs a complete modified Gram--Schmidt orthonormalization for the Cayley retraction step, replacing two cuSOLVER kernel launches (\texttt{geqr2} $+$ \texttt{orgqr}).

For the Grassmann variant, the $\bU\bU^\top$ projection is deliberately left to PyTorch's autograd (not fused into the Triton kernel) to preserve the gradient graph required by the Riemannian optimizer (\Cref{sec:grassmann}).

\subsection{CUDA Graph Compatibility}

CUDA graphs capture a fixed sequence of GPU kernels and replay them without CPU-side overhead, yielding ${\sim}3{-}5\times$ launch-overhead reduction. Several of our operations require special handling:

\paragraph{Pre-Allocated Identity Buffers.} The Cayley iteration $\bY \leftarrow \bI + \tfrac{\alpha}{2}\bW(\bI + \bY)$ requires an identity matrix $\bI \in \R^{n \times n}$. Dynamic allocation of $\bI$ via \texttt{torch.eye} breaks CUDA graph capture. We instead pre-allocate a persistent identity buffer in the module constructor:
\begin{verbatim}
self.register_buffer(
    '_I', torch.eye(n, dtype=torch.float32),
    persistent=False
)
\end{verbatim}
This buffer is registered as non-persistent (excluded from \texttt{state\_dict}) and expanded to match the batch size at runtime.

\paragraph{In-Place Scatter for Permutations.} In the Perm Mix variant, we use \texttt{torch.index\_select} (which returns a new tensor) rather than in-place scatter operations that may cause graph replay errors.

\paragraph{Static Tensor Shapes.} All projection dimensions are fixed at initialization, ensuring constant kernel configurations across forward passes.

\subsection{Distributed Data Parallelism}

\paragraph{DDP Wrapping.} All variants are compatible with both \texttt{DistributedDataParallel} (DDP) and DeepSpeed ZeRO. For our 7M-parameter model, vanilla DDP with \texttt{torch.compile(mode='default')} outperforms DeepSpeed due to lower communication overhead. All variants use only standard \texttt{nn.Parameter} tensors and register no hooks that break gradient synchronization.

\paragraph{torch.compile Integration.} Both Cayley and Sinkhorn variants are compatible with \texttt{torch.compile}. The Cayley variant's pre-allocated identity buffer (\Cref{sec:cayley}) and the Sinkhorn variant's custom \texttt{autograd.Function} are both designed to avoid dynamic tensor allocation, enabling CUDA graph capture in \texttt{reduce-overhead} mode (though \texttt{default} mode is used in production due to memory considerations).

\paragraph{Grassmannian Optimizer Integration.} The \texttt{GrassmannianOptimizer} requires access to the un-wrapped model's \texttt{GrassmannianProjection} layers. It handles both DDP and FSDP wrapping:
\begin{verbatim}
model_unwrapped = getattr(model, 'module', model)
\end{verbatim}

\paragraph{DeepSpeed ZeRO Compatibility.} All variants are validated with DeepSpeed ZeRO-2 and ZeRO-3 offloading for use with larger model configurations. The Sinkhorn custom \texttt{autograd.Function} correctly interacts with ZeRO's gradient partitioning because it only saves the output tensor $\bP$ (not intermediate buffers).

\subsection{Memory Optimization}

\paragraph{Autograd Node Reduction.} The original Sinkhorn unrolling creates $T \cdot n_{\text{ops}}$ autograd nodes per layer per sample. For $T=20$ iterations with $\sim$10 operations each, this yields $\sim$200 nodes per layer. With 6 transformer layers and 2 JPmHC modules per layer, the total is $\sim$2400 nodes. Our implicit differentiation reduces this to a \textbf{constant 1 node} per JPmHC module (12 total), a $200\times$ reduction.

\paragraph{Memory Savings.} The custom backward saves only $\bP \in \R^{B \times n \times n}$ (16 floats for $n = 4$), compared to $\sim$200 intermediate tensors for unrolled backpropagation.

\subsection{Numerical Stability}

\paragraph{Sinkhorn Log-Space.} We perform Sinkhorn iterations in log-space to avoid numerical underflow:
\begin{equation}
  \log \bP^{(t+1)}_{ij} = \bM_{ij} - \log\!\Bigl(\sum_k \exp(\bM_{ik} - r^{(t)}_i)\Bigr) - \log\!\Bigl(\sum_k \exp(\bM_{kj} - c^{(t)}_j)\Bigr),
\end{equation}
where $r^{(t)}$ and $c^{(t)}$ are running row and column normalizers.

\paragraph{Input Clamping.} Logit matrices are clamped to $[-10, 10]$ before Sinkhorn iteration to prevent \texttt{exp} overflow:
\begin{verbatim}
M = M.clamp(-10, 10)
\end{verbatim}

\paragraph{Cayley Step Size.} The Cayley alpha parameter $\alpha = 0.1$ controls the magnitude of the skew-symmetric perturbation from identity. With $s = 2$ fixed-point iterations and the iterative Cayley map, this yields orthonormality deviation $\|\bY^\top \bY - \bI\|_{\max} < 10^{-3}$ in practice.

\subsection{Trace-Based Profiling}

We use PyTorch's built-in profiler to generate Chrome-compatible trace files for analyzing compute and memory bottlenecks. From the trace files in our experiments:

\begin{table}[h]
\centering
\caption{Profiling statistics from trace analysis.}
\label{tab:trace-stats}
\begin{tabular}{lccc}
\toprule
Metric & Sinkhorn (unrolled) & Sinkhorn (implicit) & Cayley \\
\midrule
Autograd nodes per step & $\sim$128K & $\sim$1K & $\sim$1K \\
Backward time (\% of step) & $\sim$55\% & $\sim$30\% & $\sim$28\% \\
DDP sync overhead & High (stalls) & Normal & Normal \\
Trace file size (lines) & 8.9M & 4.2M & 4.2M \\
\bottomrule
\end{tabular}
\end{table}

\subsection{Registry and Factory Pattern}

We implement a variant registry to enable runtime selection of JPmHC variants via configuration:

\begin{verbatim}
_MHC_REGISTRY = {
    'sinkhorn':    MHCHyperResidualSinkhorn,
    'cayley':      MHCHyperResidualCayley,
    'grassmann':   MHCHyperResidualGrassmann,
    'spectral_gap':MHCHyperResidualSpectralGap,
    'perm_mix':    MHCHyperResidualPermMix,
}

def get_mhc_residual_class(variant: str):
    return _MHC_REGISTRY[variant]
\end{verbatim}

This allows switching between variants via a single YAML configuration flag (\texttt{mhc\_variant: perm\_mix}) without code changes.
