# Supplementary material for: JPmHC Dynamical Isometry via Orthogonal Hyper-Connections
Source: arXiv:2602.18308 source file (2026-11-08)
Supplement: Supplementary file 5 [file B_proofs_main_theorem.tex]

%!TEX root = ../rigorous_dyson_theorem.tex

\section{Proofs of Main Theorem Components (Section 3)}

This appendix contains the proofs of lemmas and propositions from Section 3, which together establish the main theorem.

\subsection{Proof of Lemma \ref{lem:stein}}
\input{rigorous_dyson_theorem/proofs/lemmas/proof_lem_stein}

\subsection{Proof of Proposition \ref{prop:self-energy}}
\input{rigorous_dyson_theorem/proofs/propositions/proof_prop_self_energy}

\subsection{Proof of Proposition \ref{prop:fixed-point}}
\input{rigorous_dyson_theorem/proofs/propositions/proof_prop_fixed_point}

\subsection{Proof of Lemma \ref{lem:concentration}}
\input{rigorous_dyson_theorem/proofs/lemmas/proof_lem_concentration}

\subsection{Proof of Theorem \ref{thm:main}}

The main theorem has four parts, proven as follows:

\textbf{Part A (Deterministic Equivalent):} The existence and uniqueness of the deterministic equivalent $\mcM(z)$ satisfying the Dyson equation follows directly from Proposition \ref{prop:fixed-point}. The scalar fixed-point formulation exploits the symmetry $m_{12} = m_{21}$ (Lemma \ref{lem:symmetry}) to reduce the problem to finding a unique $x \in \C$ satisfying $x = K(x)$, which is proven via Banach contraction mapping theorem.

\textbf{Part B (Almost Sure Convergence):} This is proven in Section 3.5 using the self-consistent error equation. The proof combines Proposition \ref{prop:self-energy} (which establishes the self-energy structure) with Lemma \ref{lem:concentration} (which provides concentration bounds). The convergence follows from showing that the error $E_N = \bTr(\E[\mcR_N]) - \bTr(\mcM)$ satisfies a contractive equation with $O(1/N)$ residual.

\textbf{Part C (Convergence Rate):} The optimal $O(1/N^2)$ convergence rate is established in Section 4 (see Theorem \ref{thm:convergence-rate} and Appendix C).

\textbf{Part D (Spectral Convergence):} This follows from Part B via the Stieltjes inversion formula (Lemma \ref{lem:stieltjes}). The almost sure convergence of $\mcG_N(z)$ to $\bTr(\mcM(z))$ implies weak convergence of the empirical spectral measure via standard arguments from random matrix theory.
