# Supplementary material for: JPmHC Dynamical Isometry via Orthogonal Hyper-Connections
Source: arXiv:2602.18308 source file (2026-11-08)
Supplement: Supplementary file 6 [file C_free_probability.tex]

%!TEX root = ../../main.tex

\section{Free Probability Tools}\label{app:free-prob}

This appendix provides the basic framework of free probability theory necessary for understanding the spectral analysis of Jacobian products in deep residual neural networks. We introduce the R-transform and S-transform, which play analogous roles to the moment and cumulant generating functions in classical probability, and explain their application to free multiplicative convolution. For comprehensive treatments, see Nica and Speicher~\cite{nica2006lectures}, Mingo and Speicher~\cite{mingo2017free}, and Hiai and Petz~\cite{hiai2000semicircle}.

\subsection{R-transform and free cumulants}

The R-transform is a fundamental tool in free probability that encodes the free cumulants of a probability distribution.

\begin{definition}[Free Cumulants and R-transform]\label{def:r-transform}
Let $\mu$ be a probability measure on $\R$ with moments $m_n = \int x^n d\mu(x)$ for $n \geq 1$. The \emph{free cumulants} $(\kappa_n)_{n \geq 1}$ of $\mu$ are defined combinatorially via non-crossing partitions (see \cite{nica2006lectures}, Lecture 11).

The \emph{R-transform} of $\mu$ is the formal power series
\begin{equation}\label{eq:r-transform-def}
\mathcal{R}_\mu(z) = \sum_{n=1}^\infty \kappa_n z^n.
\end{equation}
\end{definition}

The R-transform is related to the Cauchy (Stieltjes) transform via a functional equation.

\begin{proposition}[R-transform functional equation]\label{prop:r-cauchy-relation}
Let $G_\mu(z) = \int \frac{d\mu(\lambda)}{z - \lambda}$ be the Cauchy transform of $\mu$. Then the R-transform satisfies
\begin{equation}\label{eq:r-functional}
\mathcal{R}_\mu(G_\mu(z)) + \frac{1}{G_\mu(z)} = z.
\end{equation}

Equivalently, if $K_\mu(z) = 1/G_\mu(1/z)$ denotes the inverse Cauchy transform, then
\begin{equation}
\mathcal{R}_\mu(z) = K_\mu(z) - \frac{1}{z}.
\end{equation}
\end{proposition}

\begin{proof}[Proof sketch]
The relation \eqref{eq:r-functional} follows from the combinatorial definition of free cumulants and the moment-cumulant formula (Theorem 11.12 in \cite{nica2006lectures}). For a complete proof, see \cite{nica2006lectures}, Lecture 12.
\end{proof}

\begin{example}[Free Poisson distribution]\label{ex:free-poisson}
The free Poisson distribution with rate $\lambda > 0$ and jump size $\alpha \in \R$ has R-transform
\begin{equation}
\mathcal{R}(z) = \frac{\lambda \alpha}{1 - \alpha z}.
\end{equation}

This corresponds to the limiting spectral distribution of the matrix $\lambda^{1/2} X$, where $X$ has i.i.d.\ entries with variance $1/N$; it is the free analogue of the classical Marchenko--Pastur law~\cite{marchenko1967distribution} (see \cite{nica2006lectures}, Proposition 12.11).
\end{example}

\subsection{S-transform and multiplicative convolution}

While the R-transform linearizes free \emph{additive} convolution, the S-transform linearizes free \emph{multiplicative} convolution, making it the key tool for analyzing products of free random matrices.

\begin{definition}[S-transform]\label{def:s-transform}
Let $\mu$ be a probability measure on $\R^+$ with Cauchy transform $G_\mu(z) = \int \frac{d\mu(\lambda)}{z - \lambda}$. Define the \emph{moment function} $\Psi_\mu(z) := z\,G_\mu(z) - 1$, and let $\chi_\mu$ denote its functional inverse: $\Psi_\mu(\chi_\mu(w)) = w$. The \emph{S-transform} of $\mu$ is
\begin{equation}\label{eq:s-transform-def}
S_\mu(w) = \frac{w+1}{w \cdot \chi_\mu(w)}.
\end{equation}
Equivalently, for each $w$ in a neighborhood of~$0$, let $z_w = \chi_\mu(w)$ be the unique solution of $z\,G_\mu(z) - 1 = w$. Then
\begin{equation}\label{eq:s-transform-via-G}
S_\mu(w) = \frac{G_\mu(z_w)}{w}.
\end{equation}
\end{definition}

\begin{remark}[Reconciliation with the Cauchy--S-transform relation]
The familiar identity
\[
\frac{G(z)}{zG(z)-1} = S\bigl(zG(z)-1\bigr),
\]
is obtained by setting $w = zG(z) - 1 = \Psi(z)$ in~\eqref{eq:s-transform-via-G}. Indeed, $z_w = z$ solves $z\,G(z) - 1 = w$ by construction, so $S(w) = G(z)/w = G(z)/(zG(z)-1)$.
\end{remark}

\begin{remark}
The S-transform is particularly natural for measures on $\R^+$, which arise as the spectral distributions of $XX^T$ for random matrices $X$. For the extension to general signed measures (relevant for eigenvalues as opposed to singular values), see \cite{nica2006lectures}, Lecture 18.
\end{remark}

The key property of the S-transform is its linearization of free multiplicative convolution.

\begin{theorem}[S-transform linearization]\label{thm:s-linearization}
Let $a, b$ be freely independent random variables in a $C^*$-probability space with spectral measures $\mu_a, \mu_b$ supported on $\R^+ \cup \{0\}$. Then the spectral measure $\mu_{ab}$ of the product $ab$ satisfies
\begin{equation}\label{eq:s-multiplicative}
S_{\mu_{ab}}(z) = S_{\mu_a}(z) \cdot S_{\mu_b}(z).
\end{equation}

More generally, for a product of $L$ freely independent random variables $a_1, \ldots, a_L$,
\begin{equation}
S_{\mu_{a_1 \cdots a_L}}(z) = \prod_{l=1}^L S_{\mu_{a_l}}(z).
\end{equation}
\end{theorem}

\begin{proof}
See \cite{nica2006lectures}, Lecture 18, or \cite{voiculescu1992free} for the complete proof. The key idea is that the S-transform encodes the ``compression'' of the spectral measure under multiplication, and free independence ensures that compressions compose multiplicatively.
\end{proof}

\subsection{Free multiplicative convolution and asymptotic freeness}

\begin{definition}[Free multiplicative convolution]\label{def:free-multiplicative-convolution}
Let $\mu, \nu$ be probability measures on $\R^+$. The \emph{free multiplicative convolution} $\mu \boxtimes \nu$ is the unique probability measure on $\R^+$ whose S-transform satisfies
\begin{equation}
S_{\mu \boxtimes \nu}(z) = S_\mu(z) \cdot S_\nu(z).
\end{equation}
\end{definition}

The relevance of free multiplicative convolution to random matrix theory comes from the following fundamental result.

\begin{theorem}[Asymptotic freeness of independent matrices]\label{thm:asymptotic-freeness}
Let $A_N, B_N \in \R^{N \times N}$ be sequences of random matrices such that:
\begin{enumerate}
\item $A_N, B_N$ are independent for each $N$;
\item The empirical spectral distributions $\mu_{A_N}$ converge weakly to deterministic limits $\mu_A, \mu_B$ as $N \to \infty$;
\item Standard concentration and moment conditions hold.
\end{enumerate}

Then the empirical spectral distribution of $A_N B_N$ converges weakly to $\mu_A \boxtimes \mu_B$ as $N \to \infty$.
\end{theorem}

\begin{proof}[Proof sketch]
The key observation is that independence of matrices implies asymptotic freeness of their ``traces'' in the large-$N$ limit. This is a consequence of concentration of measure: fluctuations in $\frac{1}{N}\Tr(A_N^k B_N^l \cdots)$ become negligible, leaving only the ``free'' contributions. For a rigorous proof using subordination functions, see \cite{anderson2010introduction}, Theorem 5.4.5.
\end{proof}

\begin{corollary}[Jacobian products in ResNets]\label{cor:jacobian-free-convolution}
For a residual network with Jacobian $J = \prod_{l=1}^L Y^l$ where each $Y^l = aI + D^l W^l$ and the $W^l$ are independent random matrices, the limiting spectral measure of $J^T J$ satisfies
\begin{equation}\label{eq:jacobian-spectral}
\mu_{J^T J} = \bigboxplus_{l=1}^L \mu_{(Y^l)^T Y^l},
\end{equation}
where $\bigboxplus$ denotes the iterated free multiplicative convolution. Consequently,
\begin{equation}\label{eq:jacobian-s-transform}
S_{J^T J}(z) = \prod_{l=1}^L S_{(Y^l)^T Y^l}(z).
\end{equation}
\end{corollary}

\begin{proof}
Apply Theorem \ref{thm:asymptotic-freeness} inductively. The independence of the weight matrices $W^l$ across layers, combined with concentration of the activation patterns $D^l$, ensures that the factors $Y^l$ become asymptotically free in the large-width limit $N \to \infty$. See Section 5.1 for details.
\end{proof}

\subsection{Connection to Dyson equation and universal spectral equation}

We now connect the S-transform formalism to the Dyson equation framework of Section~\ref{sec:dyson-resnet}, and use this to derive the universal spectral equation for residual networks.

\begin{proposition}[S-transform from Dyson equation]\label{prop:s-from-dyson}
Let $Y = A + X$ where $X$ is isotropic with variance $\sigma^2/N$, and assume the deterministic equivalent $M(z)$ is given by the Dyson equation~\eqref{eq:dyson-fp}. Define the order parameters
\begin{equation}
m_{12}(z) = \frac{1}{N}\Tr(M_{12}(z)), \quad m_{21}(z) = \frac{1}{N}\Tr(M_{21}(z)).
\end{equation}

Then the S-transform of the spectral measure of $Y^\top Y$ is obtained as follows. For each $w$ in a neighborhood of $0$, let $z_w$ be the unique solution on the physical (Stieltjes) branch of
\begin{equation}\label{eq:psi-inversion-scalar}
z \, G_1(z) - 1 = w,
\end{equation}
where $G_1(z) = g_{11}(z)$ is the Cauchy transform of $Y^\top Y$ from the Dyson equation. Then
\begin{equation}\label{eq:s-from-order-params}
S_{Y^\top Y}(w) = \frac{G_1(z_w)}{w}.
\end{equation}

For the specific case $Y = aI + X$ with isotropic $X$, explicit formulas are given in \cite{tarnowski2019dynamical}, Section II.
\end{proposition}

\begin{proof}[Proof sketch]
The Cauchy transform $G(z)$ of the singular values of $Y$ is related to the (1,1) block of the resolvent via $G(z) \approx g_{11}(z) = m_{11}(z)$. The S-transform is then obtained by the change of variables in Definition \ref{def:s-transform}. The order parameters $(m_{12}, m_{21})$ encode the full spectral information through the self-consistent Dyson equation. See \cite{burda2010free} for detailed calculations in the case of products of random matrices.
\end{proof}

We can now state the main result connecting free probability to the universal spectral equation.

\begin{theorem}[Universal spectral equation via S-transform]\label{thm:universal-via-s}
Consider a deep residual network with $L$ layers, skip connection parameter $a$, and effective cumulant $c = L\sigma^2$ (Section~\ref{sec:dyson-resnet}). In the large-depth limit $L \to \infty$ with $c^l \sim c/L$ per layer, the S-transform of the Jacobian spectrum satisfies
\begin{equation}\label{eq:s-composition}
S_J(z) = \prod_{l=1}^L S_{Y^l}(z) = a^{2L} \exp\left(\int_0^z \frac{2c}{w(w+1)} dw\right) = a^{2L} \left(\frac{z+1}{z}\right)^{2c}.
\end{equation}

Inverting the S-transform to obtain the Cauchy transform $G(z)$ yields the universal equation
\begin{equation}\label{eq:universal-from-s}
\boxed{a^{2L} G(z) = (zG(z) - 1) \exp\bigl(z(1 - 2cG(z))\bigr),}
\end{equation}
which is exactly the universal spectral equation of Tarnowski et al.~\cite{tarnowski2019dynamical}.
\end{theorem}

\begin{proof}
\textbf{Step 1: S-transform composition.} By Corollary \ref{cor:jacobian-free-convolution},
\[
S_J(z) = \prod_{l=1}^L S_{Y^l}(z).
\]

For $Y^l = aI + D^l W^l$ with small random perturbations, each layer contributes approximately
\[
S_{Y^l}(z) \approx a^2 \exp\left(\frac{2c^l}{z(z+1)}\right),
\]
where $c^l$ is the effective cumulant at layer $l$ (see Proposition \ref{prop:s-from-dyson} and \cite{tarnowski2019dynamical}, Eq. (23)).

\textbf{Step 2: Large-depth limit.} Taking $L \to \infty$ with $c^l = c/L$ yields
\begin{align}
S_J(z) &= \prod_{l=1}^L a^2 \exp\left(\frac{2c/L}{z(z+1)}\right) \\
&= a^{2L} \exp\left(\sum_{l=1}^L \frac{2c/L}{z(z+1)}\right) \\
&= a^{2L} \exp\left(\frac{2c}{z(z+1)}\right) \\
&\to a^{2L} \exp\left(\int_0^z \frac{2c}{w(w+1)} dw\right) \quad \text{(continuum limit)}.
\end{align}

Evaluating the integral:
\begin{align}
\int \frac{2c}{w(w+1)} dw &= 2c \int \left(\frac{1}{w} - \frac{1}{w+1}\right) dw \\
&= 2c \log\left(\frac{w+1}{w}\right) + \text{const}.
\end{align}

Thus,
\[
S_J(z) = a^{2L} \left(\frac{z+1}{z}\right)^{2c}.
\]

\textbf{Step 3: Inversion to Cauchy transform.} We invert the S-transform using the relation $S(w) = G(z_w)/w$ where $z_w$ solves $z\,G(z) - 1 = w$ (Definition~\ref{def:s-transform}). Setting $w = z\,G_L(z) - 1$ gives $S_J(w) = G_L(z)/w$, so
\[
\frac{G_L(z)}{z\,G_L(z) - 1} = a^{2L} \left(\frac{z\,G_L(z)}{z\,G_L(z) - 1}\right)^{2c}.
\]

Let $u := z\,G_L(z)$, so $G_L(z) = u/z$ and the equation becomes
\[
\frac{u/z}{u - 1} = a^{2L} \left(\frac{u}{u - 1}\right)^{2c}.
\]

For the detailed inversion from this implicit equation to the universal form~\eqref{eq:universal-from-s}, one uses the explicit per-layer Dyson structure. Tarnowski et al.~\cite{tarnowski2019dynamical} (Section~II, Eqs.~(18)--(25)) show that the single-layer S-transform for $Y = aI + X$ with isotropic $X$ of variance $c/L$ satisfies $\log S_{Y^\top Y}(w) = 2\log a + 2(c/L)/(w(w+1)) + O(1/L^2)$. Taking the $L$-layer product and the limit $L \to \infty$ (with fixed $c$) yields
\[
a^{2L} G(z) = (zG(z) - 1) \exp\bigl(z(1 - 2cG(z))\bigr),
\]
which is the desired universal spectral equation. The detailed calculation is given in~\cite{tarnowski2019dynamical}, Eq.~(25).
\end{proof}

\begin{remark}[Universality interpretation]
Theorem \ref{thm:universal-via-s} shows that the spectral properties of the Jacobian depend \emph{only} on:
\begin{itemize}
\item The depth $L$,
\item The skip connection strength $a$,
\item The effective cumulant $c = \frac{1}{L}\sum_{l=1}^L c^l$, where $c^l$ encodes the variance and activation statistics at layer $l$.
\end{itemize}

The specific choice of activation function $\phi$ (ReLU, tanh, sigmoid, etc.) affects the spectrum \emph{only through} its contribution to $c$. This is the \textbf{spectral universality} observed in \cite{tarnowski2019dynamical}, Figure 3: different activation functions with the same effective cumulant yield identical Jacobian spectra.
\end{remark}

\begin{remark}[Dynamical isometry]
Setting $a = 1$ and solving for the value of $c$ that yields a spectrum concentrated near $\lambda = 1$ (dynamical isometry), one finds $c = 1/2$ (Definition~\ref{def:dynamical-isometry}). This critical value is universal across all activation functions, depending only on the constraint that the spectrum of $J$ should be localized at 1.
\end{remark}

\subsection{Operator-valued S-transform and Dykema's twisted multiplicativity}\label{app:ov-s-transform}

For multi-layer composition with $q > 1$, the S-transform generalises to a $\mcB$-valued map ($\mcB = M_q(\C)$). The $\mcB$-valued S-transform is $S^{(\mcB)}(W) := G^{(\mcB)}(b) \cdot W^{-1}$, where $b$ solves the \emph{Psi-inversion}
\begin{equation}\label{eq:psi-inversion}
b \cdot G^{(\mcB)}(b) - I_q = W.
\end{equation}
This inherits a \emph{twist} from the non-commutativity of $\mcB$:

\begin{theorem}[Dykema, 2006]\label{thm:dykema}
Let $x$ and $y$ be $\mcB$-freely independent positive elements. Then
\begin{equation}\label{eq:twisted-mult}
S^{(\mcB)}_{xy}(W) = S^{(\mcB)}_y(W) \cdot S^{(\mcB)}_x\!\bigl(S^{(\mcB)}_y(W)^{-1} \, W \, S^{(\mcB)}_y(W)\bigr).
\end{equation}
\end{theorem}

\noindent For $L$ layers, this gives the twisted recursion:
\begin{equation}\label{eq:twisted-fold}
S_{\mathrm{cumul}} \leftarrow S^{(\mcB)}_L(W); \quad \text{for } k = L{-}1, \ldots, 1: \;\; W_{\mathrm{tw}} = S_{\mathrm{cumul}}^{-1} W S_{\mathrm{cumul}}, \;\; S_{\mathrm{cumul}} \leftarrow S_{\mathrm{cumul}} \cdot S^{(\mcB)}_k(W_{\mathrm{tw}}).
\end{equation}
When $q = 1$, the twist is trivial (scalars commute) and~\eqref{eq:twisted-fold} reduces to $S_{\mathrm{cumul}} = \prod_l S_l(w)$.

The $L$-layer $\mcB$-valued Cauchy transform is obtained by solving the consistency equation: find $W \in M_q(\C)$ such that
\begin{equation}\label{eq:outer-consistency}
(W + I_q)\bigl(S_{\mathrm{prod}}(W) \cdot W\bigr)^{-1} = z I_q,
\end{equation}
where $S_{\mathrm{prod}}(W)$ is the twisted product~\eqref{eq:twisted-fold}. The scalar density is then $G_L(z) = \frac{1}{qz}\Tr_q(W + I_q)$.

\subsection{Scalar special case: recovery of the classical ResNet result}\label{app:scalar-recovery}

When $q = 1$ (standard residual networks with scalar skip $a$), the operator-valued Dyson equation~\eqref{eq:matrix-dyson} reduces to a scalar fixed-point problem. Together with the $z_1$-mapping for multi-layer composition, this recovers the universal spectral equation of Tarnowski et al.~\cite{tarnowski2019dynamical}.

\begin{proposition}[Scalar Dyson equation and $z_1$-mapping]\label{prop:scalar-dyson}
Let $Y = aI_N + DW$ with effective variance $\sigma^2 := \sigma_w^2\,\E[\phi'(\sqrt{q}\,Z)^2]$, $Z \sim \mathcal{N}(0,1)$.

\noindent\emph{(i) Single layer.} In the limit $N \to \infty$, the order parameter $m(z) := \frac{1}{N}\Tr\!\bigl(Y(zI_N - Y^\top\! Y)^{-1}\bigr)$ satisfies the self-consistent \emph{scalar Dyson equation}\label{app:dyson-derivation}
\begin{equation}\label{eq:dyson-fp}
m(z) = \frac{1}{N}\Tr\bigl(A_h(z)\,(zI_N - A_h(z)^\top A_h(z))^{-1}\bigr), \qquad A_h(z) := aI + \sigma^2 m(z)\, I,
\end{equation}
where $A_h$ is the dressed skip connection. The Cauchy transform is $G(z) = \frac{1}{N}\Tr(zI_N - A_h^\top A_h)^{-1}$ and the spectral density is $\rho(\lambda) = -\pi^{-1}\lim_{\eta \to 0^+}\!\Im\, G(\lambda + i\eta)$.

\noindent\emph{(ii) $L$ identical layers.}\label{prop:z1-mapping} Let $G_1(z)$ be the single-layer Cauchy transform. Then for any $z_1 \in \C^+$:
\begin{equation}\label{eq:z1-to-zL}
z_L(z_1) := z_1 \cdot \left(\frac{z_1 G_1(z_1) - 1}{G_1(z_1)}\right)^{L-1}, \qquad
G_L(z_L) = \frac{z_1 \, G_1(z_1)}{z_L}.
\end{equation}
\end{proposition}

\noindent Part~(i) is derived below via the Schwinger--Dyson approach; part~(ii) is proved in Appendix~\ref{app:z1-proof}. The Jacobian spectrum depends on $\phi$ only through the effective cumulant $c = L\sigma^2$; dynamical isometry is achieved at $c = 1/2$.

\medskip
\noindent\textbf{Derivation of part~(i).}
The argument follows the standard Schwinger--Dyson approach via Gaussian integration by parts (Appendix~\ref{app:gaussian-ibp}).

\medskip
\noindent\textbf{Step 1: Block linearization.}
Let $Y = A + X \in \R^{N \times N}$ where $A = aI_N$ is the deterministic skip and $X$ has i.i.d.\ $\mathcal{N}(0, \sigma^2/N)$ entries (the activation derivative is absorbed into $\sigma^2$ as in Section~\ref{sec:dyson-resnet}). Rather than working directly with the resolvent of $Y^\top Y$, we introduce the $2N \times 2N$ block linearization
\begin{equation}\label{eq:block-lin}
\mcL(z) = \begin{pmatrix} zI_N & -Y \\ -Y^\top & I_N \end{pmatrix},\qquad
\mcG(z) = \mcL(z)^{-1} = \begin{pmatrix} G_{11} & G_{12} \\ G_{21} & G_{22} \end{pmatrix}.
\end{equation}
By the Schur complement, the blocks of $\mcG$ encode the spectral information of $Y$:
\begin{align}
G_{11} &= (zI - YY^\top)^{-1}, \label{eq:G11}\\
G_{22} &= z\,(zI - Y^\top Y)^{-1}, \label{eq:G22}\\
G_{12} &= Y\,(zI - Y^\top Y)^{-1}. \label{eq:G12}
\end{align}
The Cauchy transform of $Y^\top Y$ is $G(z) = \frac{1}{N}\Tr(zI - Y^\top Y)^{-1} = \frac{1}{zN}\Tr G_{22}$, and the off-diagonal order parameter is $m(z) = \frac{1}{N}\Tr G_{12}$.

\medskip
\noindent\textbf{Step 2: Schwinger--Dyson equation.}
Split $\mcL = \mcL_0 + \mcV$ where
\[
\mcL_0 = \begin{pmatrix} zI & -A \\ -A^\top & I \end{pmatrix}, \qquad
\mcV = \begin{pmatrix} 0 & -X \\ -X^\top & 0 \end{pmatrix}.
\]
The identity $\mcL\,\mcG = I_{2N}$ gives $\mcG_0^{-1}\mcG + \mcV\,\mcG = I$, i.e.,
\begin{equation}\label{eq:sd-identity}
\mcG = \mcG_0 - \mcG_0 \,\mcV\, \mcG,
\end{equation}
where $\mcG_0 = \mcL_0^{-1}$ is the ``bare'' Green's function (the resolvent with $X = 0$).

\medskip
\noindent\textbf{Step 3: Wick contraction via Gaussian integration by parts.}
We take $\frac{1}{N}\Tr$ of each $N \times N$ block in~\eqref{eq:sd-identity} and take expectations. The nontrivial terms are those involving $X$ against $\mcG$. We evaluate them using Stein's lemma (Proposition~\ref{prop:matrix-stein}): for each entry $X_{ij} \sim \mathcal{N}(0, \sigma^2/N)$,
\[
\E\bigl[X_{ij}\,(\mcG)_{kl}\bigr] = \frac{\sigma^2}{N}\,\E\!\left[\frac{\partial (\mcG)_{kl}}{\partial X_{ij}}\right].
\]
The resolvent derivative (Lemma~\ref{lem:resolvent-derivative}) gives $\partial \mcG / \partial X_{ij} = \mcG \,(\partial \mcV / \partial X_{ij})\, \mcG$, so the Wick contraction produces terms quadratic in $\mcG$.

Concretely, consider the $(1,2)$ block of~\eqref{eq:sd-identity}. The term involving $X$ is $-\frac{1}{N}\Tr\bigl(\mcG_0^{(11)} X \cdot \mcG^{(22)} + \mcG_0^{(12)} X^\top \mcG^{(12)}\bigr)$, where superscripts denote $N \times N$ blocks. Taking expectations and applying Stein's lemma entry-by-entry:
\begin{align}
\E\!\left[\frac{1}{N}\sum_{i,j} X_{ij}\,(G_{22})_{ji}\right]
&= \frac{\sigma^2}{N^2}\sum_{i,j}\E\!\left[\frac{\partial (G_{22})_{ji}}{\partial X_{ij}}\right] \notag\\
&= \frac{\sigma^2}{N^2}\sum_{i,j}\E\!\left[(G_{12})_{jj}\,(G_{11})_{ii} + \cdots\right] \notag\\
&\;\xrightarrow{N \to \infty}\; \sigma^2\,m(z)\,g_{11}(z), \label{eq:wick-result}
\end{align}
where $g_{11}(z) = \lim_{N\to\infty}\frac{1}{N}\Tr G_{11}$ and $m(z) = \lim_{N\to\infty}\frac{1}{N}\Tr G_{12}$ are the deterministic limits, which exist by concentration (Theorem~\ref{thm:concentration-green}). The factorization in the last step uses the fact that $\frac{1}{N}\Tr(G_{12})$ concentrates around its expectation, so the product of traces converges to the product of limits.

The remaining Wick contractions produce analogous terms involving $m(z)$, $g_{11}(z)$, and $g_{22}(z) = z\,G(z)$.

\medskip
\noindent\textbf{Step 4: Self-consistent closure.}
Inserting the Wick contractions into the block-traced Schwinger--Dyson equation yields a closed system for the $2\times 2$ matrix of order parameters $\bigl(\begin{smallmatrix} g_{11} & m \\ \bar{m} & g_{22}\end{smallmatrix}\bigr)$. The self-energy $\sigma^2 m(z)$ enters as a scalar shift of the skip connection:
\begin{equation}\label{eq:dressed-skip}
A = aI \;\longrightarrow\; A_h(z) := aI + \sigma^2 m(z)\,I = \bigl(a + \sigma^2 m(z)\bigr)\,I.
\end{equation}
The deterministic limit of $\mcG$ equals the Green's function of the dressed block linearization
\[
\bar{\mcG}(z) = \begin{pmatrix} zI & -A_h \\ -A_h^\top & I \end{pmatrix}^{-1}\!,
\]
whose blocks are computed by the Schur complement exactly as in~\eqref{eq:G11}--\eqref{eq:G12} with $Y$ replaced by $A_h$. In particular,
\[
m(z) = \frac{1}{N}\Tr\!\bigl(A_h(zI - A_h^\top A_h)^{-1}\bigr), \qquad G(z) = \frac{1}{N}\Tr(zI - A_h^\top A_h)^{-1},
\]
which is the scalar Dyson equation~\eqref{eq:dyson-fp}. Since $A_h$ depends on $m(z)$, this is a fixed-point equation for $m$ that must be solved numerically (see Appendix~\ref{app:scalar-jacobian}).

\medskip
\noindent\textbf{Step 5: Spectral density recovery.}
Once $m(z)$ (and hence $G(z)$) has been computed on a grid $z_k = \lambda_k + i\eta$ with $\eta > 0$ small, the spectral density of $Y^\top Y$ is obtained by the Stieltjes inversion formula:
\begin{equation}\label{eq:stieltjes-inversion}
\rho(\lambda) = -\frac{1}{\pi}\lim_{\eta \to 0^+}\Im\, G(\lambda + i\eta).
\end{equation}
In practice, $\eta$ is fixed at a small positive value (the broadening parameter) and the density is read off as $\rho(\lambda) \approx -\frac{1}{\pi}\Im\, G(\lambda + i\eta)$. The singular-value density of $Y$ is then $\rho_\sigma(\sigma) = 2\sigma\,\rho(\sigma^2)$ by the change of variables $\lambda = \sigma^2$.

\subsection{Derivation of the Kronecker collapse}\label{app:kronecker-derivation}

We derive the $q \times q$ matrix Dyson equation~\eqref{eq:matrix-dyson} stated in Proposition~\ref{prop:kronecker-collapse}, extending the scalar derivation of Section~\ref{app:scalar-recovery} to the operator-valued setting.

\medskip
\noindent\textbf{Step 1: Block decomposition of $\C^N$.}
With $N = qp$ and the Kronecker skip $A = A_q \otimes I_p$, we decompose $\C^N = \C^q \otimes \C^p$. Every matrix $T \in M_N(\C)$ is viewed as a $q \times q$ array of $p \times p$ blocks:
\[
T = \bigl(T^{(\alpha\beta)}\bigr)_{\alpha,\beta=1}^q, \qquad T^{(\alpha\beta)} \in M_p(\C).
\]
The conditional expectation onto the subalgebra $\mcB = M_q(\C)$ is
\begin{equation}\label{eq:cond-exp}
E_\mcB[T] := \Bigl(\tfrac{1}{p}\Tr_p\, T^{(\alpha\beta)}\Bigr)_{\alpha,\beta=1}^q \;\in M_q(\C),
\end{equation}
which averages within each $p \times p$ sub-block while preserving the $q \times q$ block indices. The scalar trace factors as $\frac{1}{N}\Tr\, T = \frac{1}{q}\Tr_q\, E_\mcB[T]$.

\medskip
\noindent\textbf{Step 2: $\mcB$-valued order parameter.}
Define the $q \times q$ matrix-valued order parameter
\begin{equation}\label{eq:M-def}
M(z) := E_\mcB\!\bigl[Y(zI_N - Y^\top\! Y)^{-1}\bigr] = E_\mcB[G_{12}(z)] \;\in M_q(\C),
\end{equation}
where $G_{12}$ is the off-diagonal block of the $2N \times 2N$ Green's function~\eqref{eq:block-lin}. When $q = 1$, $E_\mcB$ reduces to $\frac{1}{N}\Tr$ and $M(z) = m(z)$.

\medskip
\noindent\textbf{Step 3: Wick contraction with Kronecker structure.}
We repeat the Schwinger--Dyson calculation of Section~\ref{app:scalar-recovery}, now applying $E_\mcB$ instead of $\frac{1}{N}\Tr$ to each block of~\eqref{eq:sd-identity}.

The random matrix $X = DW$ has i.i.d.\ $\mathcal{N}(0,\sigma^2/N)$ entries. The Wick contraction (Stein's lemma applied entry-by-entry as before) produces terms quadratic in the Green's function. The key structural point is that the contraction respects the $q \times q$ block decomposition:
\begin{itemize}
\item Within a given $p \times p$ sub-block $(\alpha,\beta)$, the sum over the $p^2$ entries of $X^{(\alpha\gamma)}$ paired with the resolvent produces the sub-block average $\frac{1}{p}\Tr_p(\cdot)$---exactly the $(\alpha,\gamma)$ entry of $E_\mcB[\cdot]$.
\item Across different sub-blocks, the independence of distinct entries of $X$ ensures no spurious cross-terms.
\end{itemize}
Concretely, the $(\alpha,\beta)$ component of the self-energy is:
\begin{equation}\label{eq:ov-wick}
\Sigma^{(\alpha\beta)} = \sigma^2 \sum_{\gamma=1}^q M_{\alpha\gamma}(z)\,\delta_{\gamma\beta}\, I_p
\;=\; \sigma^2\, M_{\alpha\beta}(z)\, I_p,
\end{equation}
where $M_{\alpha\beta}(z) = \frac{1}{p}\Tr_p\,(G_{12})^{(\alpha\beta)}$ is the $(\alpha,\beta)$ entry of the order parameter~\eqref{eq:M-def}. As a full $N \times N$ matrix, the self-energy is $\Sigma = \sigma^2(M(z) \otimes I_p)$: a Kronecker product that preserves the block structure.

\medskip
\noindent\textbf{Step 4: Dressed skip and $q \times q$ closure.}
The self-energy shifts the skip connection within the $q \times q$ block algebra:
\begin{equation}\label{eq:dressed-skip-ov}
A = A_q \otimes I_p \;\longrightarrow\; A_h(M) \otimes I_p, \qquad A_h(M) := A_q + \sigma^2 M(z) \;\in M_q(\C).
\end{equation}
Because $A_h(M) \otimes I_p$ is again Kronecker-structured, the dressed Green's function inherits the same block decomposition. Applying $E_\mcB$ to the Schur complement formula~\eqref{eq:G12} with $Y$ replaced by $A_h \otimes I_p$ collapses the $N \times N$ resolvent to a $q \times q$ one:
\begin{equation}\label{eq:kronecker-collapse-final}
M(z) = A_h(M)\,\bigl(zI_q - A_h(M)^\top A_h(M)\bigr)^{-1},
\end{equation}
which is the matrix Dyson equation~\eqref{eq:matrix-dyson}. The collapse works because $E_\mcB[(B \otimes I_p)(C \otimes I_p)^{-1}] = B\,C^{-1}$ for any $B, C \in M_q(\C)$ with $C$ invertible: the $p \times p$ identity factors cancel in the conditional expectation.

\medskip
\noindent\textbf{Step 5: Spectral density recovery.}
The scalar Cauchy transform of $Y^\top Y$ is
\[
G(z) = \frac{1}{q}\Tr_q\bigl(zI_q - A_h(M)^\top A_h(M)\bigr)^{-1},
\]
and the spectral density is again obtained by Stieltjes inversion~\eqref{eq:stieltjes-inversion}. The $q \times q$ equation~\eqref{eq:kronecker-collapse-final} is solved by Newton's method in $\C^{q^2}$ at cost $O(q^6)$ per step (Appendix~\ref{app:matrix-dyson-details}), compared with $O(N^3)$ for the full resolvent. Since $q \leq 4$ in practice, this is a dramatic reduction.

\begin{remark}[Verification: $q = 1$ recovery]
When $q = 1$, $A_q = a \in \R$, $M(z) = m(z) \in \C$, and~\eqref{eq:kronecker-collapse-final} becomes
\[
m = \frac{a + \sigma^2 m}{z - (a + \sigma^2 m)^2},
\]
which is exactly~\eqref{eq:dyson-fp} evaluated for $A_h = (a + \sigma^2 m)\,I_N$.
\end{remark}
