# Supplementary material for: JPmHC Dynamical Isometry via Orthogonal Hyper-Connections
Source: arXiv:2602.18308 source file (2026-11-08)
Supplement: Supplementary file 7 [file D_technical_lemmas.tex]

%!TEX root = ../../rigorous_dyson_theorem.tex

\section{Technical Lemmas}

This appendix collects technical results on Herglotz functions, Schur complements, trace inequalities, and resolvent calculus that are referenced throughout the main proofs. These results are standard in random matrix theory but are included here for completeness.

\subsection{Herglotz function properties}

\begin{lemma}[Herglotz function characterization]\label{lem:herglotz-char}
A function $f: \C^+ \to \C$ is a Herglotz function (i.e., analytic and maps $\C^+ \to \C^+$) if and only if it can be represented as
\[
f(z) = \alpha z + \beta + \int_\R \frac{1 + \lambda z}{z - \lambda} d\nu(\lambda),
\]
where $\alpha \geq 0$, $\beta \in \R$, and $\nu$ is a finite positive measure on $\R$ satisfying $\int_\R \frac{d\nu(\lambda)}{1 + \lambda^2} < \infty$.
\end{lemma}

\begin{proof}
This is the Nevanlinna representation theorem. See \cite{anderson2010introduction}, Appendix A.2, for a complete proof.
\end{proof}

\subsection{Schur complement formulas}

\begin{lemma}[General Schur complement]\label{lem:schur-general}
Let $M = \begin{pmatrix} A & B \\ C & D \end{pmatrix}$ be a block matrix with invertible blocks $A, D$. Then:
\begin{enumerate}
\item $M$ is invertible if and only if the Schur complement $S_A = D - CA^{-1}B$ is invertible
\item When $M$ is invertible,
\[
M^{-1} = \begin{pmatrix} (A - BD^{-1}C)^{-1} & -A^{-1}B(D - CA^{-1}B)^{-1} \\
-D^{-1}C(A - BD^{-1}C)^{-1} & (D - CA^{-1}B)^{-1} \end{pmatrix}
\]
\item $\det(M) = \det(A) \det(S_A) = \det(D) \det(S_D)$, where $S_D = A - BD^{-1}C$
\end{enumerate}
\end{lemma}

\begin{proof}
Standard linear algebra result. For (1)-(2), use block Gaussian elimination. For (3), compute the determinant after factorizing $M = \begin{pmatrix} I & 0 \\ CA^{-1} & I \end{pmatrix} \begin{pmatrix} A & B \\ 0 & S_A \end{pmatrix}$.
\end{proof}

\subsection{Trace inequalities}

\begin{lemma}[Trace Cauchy-Schwarz]\label{lem:trace-cs}
For any matrices $A, B \in \C^{N \times N}$,
\[
|\Tr(AB)| \leq \sqrt{\Tr(A^\dagger A)} \cdot \sqrt{\Tr(B^\dagger B)} = \norm{A}_F \norm{B}_F.
\]
\end{lemma}

\begin{proof}
This follows from the Cauchy-Schwarz inequality applied to the Frobenius inner product $\langle A, B \rangle = \Tr(A^\dagger B)$.
\end{proof}

\begin{lemma}[Trace submultiplicativity]\label{lem:trace-submult}
For any matrices $A, B \in \R^{N \times N}$ with $A, B \succeq 0$ (positive semidefinite),
\[
\Tr(AB) \leq \norm{A} \Tr(B) = \norm{B} \Tr(A).
\]
\end{lemma}

\begin{proof}
Let $\lambda_1 \geq \lambda_2 \geq \cdots \geq \lambda_N$ be the eigenvalues of $A$. Then $\norm{A} = \lambda_1$ and
\[
\Tr(AB) = \sum_i \lambda_i(AB) \leq \lambda_1 \sum_i \mathbb{1}_{\{\lambda_i(B) \geq 0\}} \lambda_i(B) \leq \lambda_1 \Tr(B).
\]
\end{proof}

\subsection{Resolvent derivative bounds}

\begin{lemma}[Resolvent derivative formula]\label{lem:resolvent-derivative}
Let $R(z) = (zI - H)^{-1}$ for a self-adjoint matrix $H$. For any $k, l \in \{1, \ldots, N\}$ and matrix entry $H_{ij}$,
\[
\frac{\partial R_{kl}}{\partial H_{ij}} = -(R e_i e_j^\top R)_{kl} = -\sum_p R_{kp} (e_i e_j^\top)_{pm} R_{ml} = -R_{ki} R_{jl}.
\]
\end{lemma}

\begin{proof}
Differentiate the identity $(zI - H)R(z) = I$ with respect to $H_{ij}$:
\[
-(\partial_{H_{ij}} H) R + (zI - H) \partial_{H_{ij}} R = 0.
\]
Since $\partial_{H_{ij}} H = e_i e_j^\top$, we have
\[
\partial_{H_{ij}} R = R (e_i e_j^\top) R.
\]
Extracting the $(k, l)$ entry gives the result.
\end{proof}

\begin{lemma}[Resolvent Lipschitz constant]\label{lem:resolvent-lipschitz}
For $z \in \C^+$ with $\Im(z) \geq \eta > 0$, the resolvent $R(z) = (zI - H)^{-1}$ satisfies
\[
\norm{\frac{\partial R}{\partial H_{ij}}}_F \leq \frac{1}{\eta^2}.
\]
\end{lemma}

\begin{proof}
From Lemma \ref{lem:resolvent-derivative},
\[
\left\|\frac{\partial R}{\partial H_{ij}}\right\|_F = \norm{R e_i e_j^\top R}_F \leq \norm{R}^2 \norm{e_i e_j^\top}_F = \norm{R}^2 \leq \frac{1}{\eta^2}.
\]
This bound is tight and does not require additional factors.
\end{proof}

\begin{remark}
These technical results are used throughout the concentration inequalities (Appendix B) and the main convergence proofs (Section 3). The resolvent derivative bounds are particularly crucial for applying Poincaré's inequality and bounding variance terms.
\end{remark}
