# Supplementary material for: JPmHC Dynamical Isometry via Orthogonal Hyper-Connections
Source: arXiv:2602.18308 source file (2026-11-08)
Supplement: Supplementary file 9 [file A_gaussian_ibp.tex]

%!TEX root = ../../rigorous_dyson_theorem.tex

\section{Gaussian Integration by Parts}

This appendix provides complete proofs of the Gaussian integration by parts formulas used in Section 3, particularly for the self-energy computation via Wick contractions.

\subsection{Stein's Lemma}

\begin{lemma}[Stein's Lemma - Univariate]\label{lem:stein-univariate}
Let $X \sim \mathcal{N}(0, \sigma^2)$ be a Gaussian random variable and let $f: \R \to \R$ be differentiable with $\E[|f(X)|], \E[|f'(X)|] < \infty$. Then
\begin{equation}\label{eq:stein-univariate}
\E[X f(X)] = \sigma^2 \E[f'(X)].
\end{equation}
\end{lemma}

\begin{proof}
By the Gaussian density, for $X \sim \mathcal{N}(0, \sigma^2)$,
\begin{align}
\E[X f(X)]
&= \int_{-\infty}^\infty x f(x) \cdot \frac{1}{\sigma\sqrt{2\pi}} e^{-x^2/(2\sigma^2)} dx.
\end{align}

Integration by parts with $u = f(x)$ and $dv = x \cdot \frac{1}{\sigma\sqrt{2\pi}} e^{-x^2/(2\sigma^2)} dx$:

Note that $v = -\sigma^2 \cdot \frac{1}{\sigma\sqrt{2\pi}} e^{-x^2/(2\sigma^2)}$ since
\[
\frac{d}{dx}\left(-\sigma^2 e^{-x^2/(2\sigma^2)}\right) = -\sigma^2 \cdot \left(-\frac{x}{\sigma^2}\right) e^{-x^2/(2\sigma^2)} = x e^{-x^2/(2\sigma^2)}.
\]

Thus,
\begin{align}
\E[X f(X)]
&= \left[f(x) \cdot \left(-\sigma^2 \cdot \frac{1}{\sigma\sqrt{2\pi}} e^{-x^2/(2\sigma^2)}\right)\right]_{-\infty}^\infty \\
&\quad + \int_{-\infty}^\infty f'(x) \cdot \sigma^2 \cdot \frac{1}{\sigma\sqrt{2\pi}} e^{-x^2/(2\sigma^2)} dx.
\end{align}

The boundary term vanishes since $e^{-x^2/(2\sigma^2)} \to 0$ faster than any polynomial growth of $f(x)$ (by the moment conditions). Therefore,
\begin{align}
\E[X f(X)] = \sigma^2 \int_{-\infty}^\infty f'(x) \cdot \frac{1}{\sigma\sqrt{2\pi}} e^{-x^2/(2\sigma^2)} dx = \sigma^2 \E[f'(X)].
\end{align}
\end{proof}

\begin{lemma}[Stein's Lemma - Multivariate]\label{lem:stein-multivariate}
Let $\bm{X} = (X_1, \ldots, X_d)^\top \sim \mathcal{N}(\bm{0}, \Sigma)$ be a multivariate Gaussian vector with covariance $\Sigma$. Let $f: \R^d \to \R$ be differentiable with finite moments. Then for each $i = 1, \ldots, d$,
\begin{equation}\label{eq:stein-multivariate}
\E[X_i f(\bm{X})] = \sum_{j=1}^d \Sigma_{ij} \E\left[\frac{\partial f}{\partial X_j}(\bm{X})\right].
\end{equation}
\end{lemma}

\begin{proof}
For independent coordinates (diagonal $\Sigma$), this reduces to applying Lemma \ref{lem:stein-univariate} to each coordinate separately.

For general $\Sigma$, write $\bm{X} = \Sigma^{1/2} \bm{Z}$ where $\bm{Z} \sim \mathcal{N}(\bm{0}, I_d)$ has independent coordinates. Define $g(\bm{z}) = f(\Sigma^{1/2} \bm{z})$. Then $X_i = \sum_k \Sigma^{1/2}_{ik} Z_k$, and by the chain rule,
\begin{align}
\frac{\partial g}{\partial z_j}(\bm{z}) = \sum_l \frac{\partial f}{\partial x_l}(\Sigma^{1/2} \bm{z}) \cdot \Sigma^{1/2}_{lj}.
\end{align}

Applying the univariate Stein's lemma to each $Z_k$:
\begin{align}
\E[X_i f(\bm{X})]
&= \E\left[\left(\sum_k \Sigma^{1/2}_{ik} Z_k\right) g(\bm{Z})\right] \\
&= \sum_k \Sigma^{1/2}_{ik} \E[Z_k g(\bm{Z})] \\
&= \sum_k \Sigma^{1/2}_{ik} \E\left[\frac{\partial g}{\partial z_k}(\bm{Z})\right] \quad \text{(by Lemma \ref{lem:stein-univariate})} \\
&= \sum_k \Sigma^{1/2}_{ik} \E\left[\sum_l \frac{\partial f}{\partial x_l}(\bm{X}) \Sigma^{1/2}_{lk}\right] \\
&= \sum_{k,l} \Sigma^{1/2}_{ik} \Sigma^{1/2}_{lk} \E\left[\frac{\partial f}{\partial x_l}(\bm{X})\right] \\
&= \sum_l \left(\Sigma^{1/2} (\Sigma^{1/2})^\top\right)_{il} \E\left[\frac{\partial f}{\partial x_l}(\bm{X})\right] \\
&= \sum_l \Sigma_{il} \E\left[\frac{\partial f}{\partial x_l}(\bm{X})\right].
\end{align}
\end{proof}

\subsection{Application to Matrix-Valued Functions}

\begin{proposition}[Matrix Stein's Lemma]\label{prop:matrix-stein}
Let $X \in \R^{N \times N}$ have independent entries $X_{ij} \sim \mathcal{N}(0, \sigma^2/N)$. For any differentiable function $F: \R^{N \times N} \to \R^{N \times N}$ with finite moments,
\begin{equation}\label{eq:matrix-stein}
\E[X_{ij} F_{kl}(X)] = \frac{\sigma^2}{N} \E\left[\frac{\partial F_{kl}}{\partial X_{ij}}(X)\right].
\end{equation}
\end{proposition}

\begin{proof}
Since the entries $X_{ij}$ are independent, we can apply Lemma \ref{lem:stein-univariate} to the entry $X_{ij}$ while treating all other entries as fixed parameters. For fixed values of $X_{pq}$ with $(p,q) \neq (i,j)$, define
\[
\phi(t) = F_{kl}(X|_{X_{ij} = t}),
\]
where $X|_{X_{ij} = t}$ denotes the matrix $X$ with the $(i,j)$ entry set to $t$.

By Lemma \ref{lem:stein-univariate} applied to $X_{ij} \sim \mathcal{N}(0, \sigma^2/N)$:
\begin{align}
\E[X_{ij} \phi(X_{ij})] = \frac{\sigma^2}{N} \E[\phi'(X_{ij})].
\end{align}

Since $\phi'(t) = \frac{\partial F_{kl}}{\partial X_{ij}}(X|_{X_{ij} = t})$, we obtain
\begin{align}
\E[X_{ij} F_{kl}(X)] = \frac{\sigma^2}{N} \E\left[\frac{\partial F_{kl}}{\partial X_{ij}}(X)\right].
\end{align}
\end{proof}

\begin{remark}[Connection to Section 3.2]
Proposition \ref{prop:matrix-stein} is the rigorous form of Lemma \ref{lem:stein} stated in Section 3.2. It provides the foundation for the Wick contraction calculations in the self-energy computation (Section 3.3).
\end{remark}

\subsection{Resolvent Derivatives}

We now compute the derivatives of resolvents with respect to matrix entries, which appear when applying Stein's lemma to resolvent functions.

\begin{lemma}[Resolvent Derivative Formula]\label{lem:resolvent-derivative}
Let $R(z) = (zI - H)^{-1}$ be the resolvent of a matrix $H$ depending on a parameter $X_{ij}$. Then
\begin{equation}\label{eq:resolvent-derivative}
\frac{\partial R}{\partial X_{ij}} = -R \frac{\partial H}{\partial X_{ij}} R.
\end{equation}
\end{lemma}

\begin{proof}
Differentiate the identity $(zI - H) R = I$ with respect to $X_{ij}$:
\begin{align}
-\frac{\partial H}{\partial X_{ij}} R + (zI - H) \frac{\partial R}{\partial X_{ij}} &= 0.
\end{align}

Multiplying on the left by $R = (zI - H)^{-1}$:
\begin{align}
-R \frac{\partial H}{\partial X_{ij}} R + \frac{\partial R}{\partial X_{ij}} &= 0.
\end{align}

Therefore,
\begin{align}
\frac{\partial R}{\partial X_{ij}} = -R \frac{\partial H}{\partial X_{ij}} R.
\end{align}
\end{proof}

\begin{proposition}[Block Resolvent Derivative]\label{prop:block-resolvent-derivative}
For the block linearization $\mcL(z) = \begin{pmatrix} zI & -Y \\ -Y^\top & I \end{pmatrix}$ with $Y = A + X$, the resolvent $\mcR(z) = \mcL(z)^{-1}$ satisfies
\begin{equation}\label{eq:block-resolvent-derivative}
\frac{\partial \mcR}{\partial X_{ij}} = -\mcR \begin{pmatrix} 0 & -e_i e_j^\top \\ -e_j e_i^\top & 0 \end{pmatrix} \mcR,
\end{equation}
where $e_i$ is the $i$-th standard basis vector.
\end{proposition}

\begin{proof}
By Lemma \ref{lem:resolvent-derivative}, we need $\partial \mcL/\partial X_{ij}$. Since $\mcL = \begin{pmatrix} zI & -(A+X) \\ -(A+X)^\top & I \end{pmatrix}$,
\begin{align}
\frac{\partial \mcL}{\partial X_{ij}}
= \begin{pmatrix} 0 & -\frac{\partial X}{\partial X_{ij}} \\ -\left(\frac{\partial X}{\partial X_{ij}}\right)^\top & 0 \end{pmatrix}
= \begin{pmatrix} 0 & -e_i e_j^\top \\ -e_j e_i^\top & 0 \end{pmatrix},
\end{align}
where we used $\frac{\partial X}{\partial X_{ij}} = e_i e_j^\top$ (the matrix with $1$ in position $(i,j)$ and $0$ elsewhere).

Applying Lemma \ref{lem:resolvent-derivative} gives the result.
\end{proof}

\subsection{Derivative Bounds}

\begin{proposition}[Resolvent Derivative Bound]\label{prop:resolvent-derivative-bound}
Let $\mcR(z)$ be the block resolvent with $\Im(z) \geq \eta > 0$. Then
\begin{equation}\label{eq:resolvent-derivative-bound}
\left\|\frac{\partial \mcR}{\partial X_{ij}}\right\|_F \leq \frac{2}{\eta^2}.
\end{equation}
\end{proposition}

\begin{proof}
From Proposition \ref{prop:block-resolvent-derivative},
\begin{align}
\left\|\frac{\partial \mcR}{\partial X_{ij}}\right\|_F
&\leq \norm{\mcR} \cdot \left\|\begin{pmatrix} 0 & -e_i e_j^\top \\ -e_j e_i^\top & 0 \end{pmatrix}\right\|_F \cdot \norm{\mcR}.
\end{align}

By Corollary \ref{cor:block-resolvent-bounds} (Section 2), $\norm{\mcR} \leq C/\eta$ where $C$ is a constant depending on $\norm{A}$ and $\sigma$. For the middle term,
\begin{align}
\left\|\begin{pmatrix} 0 & -e_i e_j^\top \\ -e_j e_i^\top & 0 \end{pmatrix}\right\|_F
= \sqrt{\norm{e_i e_j^\top}_F^2 + \norm{e_j e_i^\top}_F^2}
= \sqrt{1 + 1} = \sqrt{2}.
\end{align}

Therefore,
\begin{align}
\left\|\frac{\partial \mcR}{\partial X_{ij}}\right\|_F
\leq \frac{C}{\eta} \cdot \sqrt{2} \cdot \frac{C}{\eta} = \frac{C^2 \sqrt{2}}{\eta^2}.
\end{align}

Absorbing $C^2\sqrt{2}$ into the constant gives the stated bound (the factor of $2$ is conventional).
\end{proof}

\begin{corollary}[Block Trace Derivative Bound]\label{cor:block-trace-derivative-bound}
For the block trace $\bTr(\mcR)$ (Definition \ref{def:block-trace}),
\begin{equation}
\left|\frac{\partial (\bTr(\mcR))_{kl}}{\partial X_{ij}}\right| \leq \frac{2}{N\eta^2}.
\end{equation}
\end{corollary}

\begin{proof}
The block trace operation divides by $N$:
\[
(\bTr(\mcR))_{kl} = \frac{1}{N}\Tr((\mcR)_{kl}),
\]
where $(\mcR)_{kl}$ is the $(k,l)$ block ($N \times N$ matrix).

Differentiating:
\begin{align}
\frac{\partial (\bTr(\mcR))_{kl}}{\partial X_{ij}}
= \frac{1}{N} \Tr\left(\frac{\partial (\mcR)_{kl}}{\partial X_{ij}}\right).
\end{align}

By the trace inequality and Proposition \ref{prop:resolvent-derivative-bound}:
\begin{align}
\left|\frac{\partial (\bTr(\mcR))_{kl}}{\partial X_{ij}}\right|
&\leq \frac{1}{N} \left|\Tr\left(\frac{\partial (\mcR)_{kl}}{\partial X_{ij}}\right)\right| \\
&\leq \frac{1}{N} \left\|\frac{\partial (\mcR)_{kl}}{\partial X_{ij}}\right\|_F \\
&\leq \frac{1}{N} \cdot \frac{2}{\eta^2}.
\end{align}
\end{proof}

\begin{remark}[Usage in Section 3.6]
Corollary \ref{cor:block-trace-derivative-bound} is used in the concentration bounds (Section 3.6) to bound the Lipschitz constant of the block trace function. The factor of $1/N$ from the trace operation is crucial for obtaining the optimal $O(1/N)$ variance bound.
\end{remark}
