# Supplementary material for: JPmHC Dynamical Isometry via Orthogonal Hyper-Connections
Source: arXiv:2602.18308 source file (2026-11-08)
Supplement: Supplementary file 10 [file A_proofs_preliminaries.tex]

%!TEX root = ../rigorous_dyson_theorem.tex

\section{Proofs of Preliminaries (Section 2)}

This appendix contains the proofs of all lemmas and corollaries from Section 2 (Preliminaries).

\subsection{Proof of Lemma \ref{lem:resolvent-identity}}
\input{rigorous_dyson_theorem/proofs/lemmas/proof_lem_resolvent_identity}

\subsection{Proof of Lemma \ref{lem:resolvent-bounds}}
\input{rigorous_dyson_theorem/proofs/lemmas/proof_lem_resolvent_bounds}

\subsection{Proof of Corollary \ref{cor:block-resolvent-bounds}}
\input{rigorous_dyson_theorem/proofs/corollaries/proof_cor_block_resolvent_bounds}

\subsection{Proof of Lemma \ref{lem:isotropy-moments}}
\input{rigorous_dyson_theorem/proofs/lemmas/proof_lem_isotropy_moments}

\subsection{Proof of Lemma \ref{lem:stieltjes}}
\input{rigorous_dyson_theorem/proofs/lemmas/proof_lem_stieltjes}

\subsection{Proof of Lemma \ref{lem:schur}}
\input{rigorous_dyson_theorem/proofs/lemmas/proof_lem_schur}

\subsection{Proof of Lemma \ref{lem:block-inversion}}
\input{rigorous_dyson_theorem/proofs/lemmas/proof_lem_block_inversion}

\subsection{Proof of Lemma \ref{lem:symmetry}}
\input{rigorous_dyson_theorem/proofs/lemmas/proof_lem_symmetry}
