# Supplementary material for: JPmHC Dynamical Isometry via Orthogonal Hyper-Connections
Source: arXiv:2602.18308 source file (2026-11-08)
Supplement: Supplementary file 11 [file C_proofs_convergence.tex]

%!TEX root = ../rigorous_dyson_theorem.tex

\section{Proofs of Convergence Rate Results (Section 4)}

This appendix contains the proof of the convergence rate theorem from Section 4.

\subsection{Proof of Theorem \ref{thm:convergence-rate}}
\input{rigorous_dyson_theorem/proofs/theorems/proof_thm_convergence_rate}
