# Supplementary material for: JPmHC Dynamical Isometry via Orthogonal Hyper-Connections
Source: arXiv:2602.18308 source file (2026-11-08)
Supplement: Supplementary file 12 [file D_proofs_introduction.tex]

%!TEX root = ../rigorous_dyson_theorem.tex

\section{Proofs of Introduction Results (Section 1)}

This appendix contains proofs of the corollaries stated in Section 1.

\subsection{Proof of Corollary \ref{cor:scalar}}
\input{rigorous_dyson_theorem/proofs/corollaries/proof_cor_scalar}

\subsection{Proof of Corollary \ref{cor:universality}}
\input{rigorous_dyson_theorem/proofs/corollaries/proof_cor_universality}
