# Supplementary material for: JPmHC Dynamical Isometry via Orthogonal Hyper-Connections
Source: arXiv:2602.18308 source file (2026-11-08)
Supplement: Supplementary file 13 [file E_proofs_applications.tex]

%!TEX root = ../rigorous_dyson_theorem.tex

\section{Proofs for Application to Residual Networks (Section 5)}

This appendix contains proofs of the propositions, theorems, and corollaries from Section 5 on applications to residual neural networks.

\subsection{Proof of Proposition \ref{prop:layerwise}}
\input{rigorous_dyson_theorem/proofs/propositions/proof_prop_layerwise}

\subsection{Proof of Theorem \ref{thm:universal-resnet}}
\input{rigorous_dyson_theorem/proofs/theorems/proof_thm_universal_resnet}

\subsection{Proof of Corollary \ref{cor:dynamical-isometry}}
\input{rigorous_dyson_theorem/proofs/corollaries/proof_cor_dynamical_isometry}
